# Supplementary material for: Byzantine-Robust and Privacy-Preserving Framework for FedML
Source: arXiv:2105.02295 source file (2021-05-05)
Supplement: Supplementary file 1 [file 2Appendix.tex]

\section{Privacy}
\begin{thm}\label{thm:bound_sum}
Assume that $\mathbf x\sim P_x$ $(\mathbf x\in\mathbb R^d)$ is a random vector, and $R\sim \mathcal N(\mu,\sigma^2\mathbb I)$ is a Gaussian random vector with covariance $\sigma^2\mathbb I$ and mean $\mu$. Then we have,
\begin{align}
    I(\mathbf x;\mathbf x+R)\leq \sum_{i=1}^d\frac{\text{Var}(\mathbf{x}_i)}{\sigma^2}~,
\end{align}
where $\text{Var}(\mathbf{x}_i)$ is variance of the $i$th entry of the random variable $\mathbf x$.
\end{thm}
\begin{proof}
Because $\mu$ is fixed and so $I(\mathbf x;\mathbf x+R)=I(\mathbf x;\mathbf x+R-\mu)$, without loss of generality, we assume that $\mu=0$. Define the random variable $Z$ to be $Z=\mathbf x+R$, and let $f_X(\cdot)$ and $f_Z(\cdot)$ to be the probability density function of the random variables $\mathbf x$ and $Z$, respectively. Also let $\phi(x)=\frac{1}{\sqrt{2\pi}}e^{-\|x\|^2/2}$ to be the probability density function of a standard Gaussian random variable. \\
We are interested in 
\begin{align}\label{eq:def_mi_pf}
    I(\mathbf x;\mathbf x+R)=I(X;Z)=H(Z)-H(R)~.
\end{align}
Since $R$ is a zero-mean Gaussian random variables with variance $\sigma^2$, we have
\begin{align}\label{eq:entropy_Gaussian}
    H(R)=\frac{d}{2} \log(2\pi e \sigma^2)~.
\end{align}
It remains to bound $H(z)$ in \eqref{eq:def_mi_pf}. Note that the probability distribution function of $Z$, $f_Z(\cdot)$, will be
\begin{align}
    f_{Z}(t)=\int_{-\infty}^\infty f_X(x)\frac{1}{\sigma}\phi\left( \frac{x-t}{\sigma} \right)~dx=\mathbb{E}_{x\sim P_X}\left[\frac{1}{\sigma}\phi\left(\frac{x-t}{\sigma}\right) \right]~
\end{align}
where the last expected value is over the distribution of $X$. Now that we have pdf of the random variable $Z$, we can calculate and bound its entropy as follows,
%\resizebox{.9\linewidth}{!}{
%\begin{small}
\begin{align}\label{eq:apply_jensen}
    &H(Z)=-\int f_Z(z)\log\left(f_Z(z)\right)~dz\nonumber\\
    &=-\int \mathbb{E}_{x_1}\left[\frac{1}{\sigma}\phi\left(\frac{x_1-z}{\sigma}\right)\right]\log\left(\mathbb{E}_{x_2}\left[\frac{1}{\sigma}\phi\left(\frac{x_2-z}{\sigma}\right) \right]\right)dz\nonumber\\
    &\leq -\int \mathbb{E}_{x_1}\left[\frac{1}{\sigma}\phi\left(\frac{x_1-z}{\sigma}\right) \right]\mathbb{E}_{x_2}\left[\log\left(\frac{1}{\sigma}\phi\left(\frac{x_2-z}{\sigma}\right) \right)\right]dz\nonumber\\
    &=\mathbb{E}_{x_1,x_2\sim P_X}\left[ -\int \frac{1}{\sigma}\phi\left(\frac{x_1-z}{\sigma}\right) \log\left(\frac{1}{\sigma}\phi\left(\frac{x_2-z}{\sigma}\right) \right)dz \right].
\end{align}
%\end{small}
The only inequality in the equations above is due to Jensen's inequality (since $-\log(x)$ is a convex function). Now we can explicitly calculate the integral in the last line of \eqref{eq:apply_jensen} (as they are all Gaussian integrals).
\begin{align}\label{eq:Gaussian_int}
    -\int \frac{1}{\sigma}\phi\left(\frac{x_1-z}{\sigma}\right) \log\left(\frac{1}{\sigma}\phi\left(\frac{x_2-z}{\sigma}\right) \right)~dz\nonumber\\
    =\frac d 2 \log(2\pi e \sigma^2)+\frac{1}{2\sigma^2}\|x_1-x_2\|^2~.
\end{align}
Combining \eqref{eq:Gaussian_int} and \eqref{eq:apply_jensen} bounds $H(Z)$ as desired,
\begin{align}\label{eq:bound_z}
    H(Z)\leq \mathbb{E}_{x_1,x_2\sim P_X}\left[  \frac 1 2 \log(2\pi e \sigma^2)+\frac{1}{2\sigma^2}\|x_1-x_2\|^2\right]\nonumber\\
    =\frac d 2 \log(2\pi e \sigma^2)+\sum_{i=1}^d\frac{\text{Var}(\mathbf{x}_i)}{\sigma^2}~.
\end{align}
Finally, combining \eqref{eq:def_mi_pf}, \eqref{eq:entropy_Gaussian} and \eqref{eq:bound_z} yields
\begin{align}
    I(X;X+R)&\leq \frac d 2 \log(2\pi e \sigma^2)+\sum_{i=1}^d\frac{\text{Var}(\mathbf{x}_i)}{\sigma^2}-\frac d 2 \log(2\pi e \sigma^2)\nonumber\\
    &=\sum_{i=1}^d\frac{\text{Var}(\mathbf{x}_i)}{\sigma^2}~,
\end{align}
which concludes the proof.
\end{proof}
